# Supplementary material for: The cycling mechanism of manganese-oxide cathodes in zinc batteries: A theory-based approach
Source: arXiv:2308.03352 ancillary file (2023-08-07)
Supplement: Supplementary file 1 [file SupportingInformation.pdf]

# Supporting Information: The cycling mechanism of manganese-oxide cathodes in zinc batteries: A theory-based approach

Niklas J. Herrmann,[†,‡,¶] Holger Euchner,[¶,§] Axel Groß,[¶,‡] and Birger Horstmann[*,†,‡,¶]

†*German Aerospace Center, Wilhelm-Runge-Straße 10, D-89081 Ulm, Germany*

‡*Helmholtz Institute Ulm, Helmholtzstraße 11, D-89081 Ulm, Germany*

¶*Universität Ulm, Albert-Einstein-Allee 47, D-89081 Ulm, Germany*

§*University of Tübingen, Auf der Morgenstelle 18, D-72076 Tübingen, Germany*

E-mail: birger.horstmann@dlr.de

# Contents

**1 Model details** **S-3**

1.1 Electrolyte Thermodynamics . . . . . . . . . . . . . . . . . . . . . . . . . . . . S-3

1.2 Cathode Thermodynamics . . . . . . . . . . . . . . . . . . . . . . . . . . . . S-6

1.3 Continuum Model . . . . . . . . . . . . . . . . . . . . . . . . . . . . . . . . S-8

1.4 Cathode Model . . . . . . . . . . . . . . . . . . . . . . . . . . . . . . . . . S-8

**2 Cell Parametrization** **S-10**

**3 Simulation Result** **S-13**

3.1 Electrolyte Speciation (Thermodynamics) . . . . . . . . . . . . . . . . . . . . S-14

3.2 Electrode Thermodynamics (DFT) . . . . . . . . . . . . . . . . . . . . . . . S-15

3.3 Proton insertion in the first phase (Cell Model) . . . . . . . . . . . . . . . . . S-17

3.4 Cell-level simulations . . . . . . . . . . . . . . . . . . . . . . . . . . . . . S-19

**References** **S-22**

# 1 Model details

## 1.1 Electrolyte Thermodynamics

**Table S1: Complex formation reactions in the electrolyte and the corresponding thermodynamic stability constants. Data from References S1–S4**

| Reaction | $\log_{10}\beta$ |
|---|---|
| $H^+ + OH^- \rightleftharpoons H_2O$ | −14.0 |
| $2\,H^+ + SO_4{}^{2-} \rightleftharpoons H_2SO_4$ | 0.0 |
| $H^+ + SO_4{}^{2-} \rightleftharpoons HSO_4{}^-$ | 1.98 |
| $Zn^{2+} + H_2O \rightleftharpoons ZnOH^+ + H^+$ | −7.5 |
| $Zn^{2+} + 2\,H_2O \rightleftharpoons Zn(OH)_2 + 2\,H^+$ | −16.4 |
| $Zn^{2+} + 3\,H_2O \rightleftharpoons Zn(OH)_3{}^- + 3\,H^+$ | −28.2 |
| $Zn^{2+} + 4\,H_2O \rightleftharpoons Zn(OH)_4{}^{2-} + 4\,H^+$ | −41.3 |
| $2\,Zn^{2+} + H_2O \rightleftharpoons Zn_2OH^{3+} + H^+$ | −9 |
| $2\,Zn^{2+} + 6\,H_2O \rightleftharpoons Zn_2(OH)_6{}^{2-} + 6\,H^+$ | −54.3 |
| $4\,Zn^{2+} + 4\,H_2O \rightleftharpoons Zn_4(OH)_4{}^{4+} + 4\,H^+$ | −27.0 |
| $Zn^{2+} + SO_4{}^{2-} \rightleftharpoons ZnSO_4$ | 2.37 |
| $Zn^{2+} + 2\,SO_4{}^{2-} \rightleftharpoons Zn(SO_4)_2{}^{2-}$ | 3.28 |
| $Zn^{2+} + 3\,SO_4{}^{2-} \rightleftharpoons Zn(SO_4)_3{}^{4-}$ | 1.7 |
| $Zn^{2+} + 4\,SO_4{}^{2-} \rightleftharpoons Zn(SO_4)_4{}^{6-}$ | 1.7 |
| $Mn^{2+} + H_2O \rightleftharpoons Mn(OH)^+ + H^+$ | −10.59 |
| $Mn^{2+} + 2\,H_2O \rightleftharpoons Mn(OH)_2 + 2\,H^+$ | −18.54 |
| $Mn^{2+} + 3\,H_2O \rightleftharpoons Mn(OH)_3{}^- + 3\,H^+$ | −34.8 |
| $Mn^{2+} + 4\,H_2O \rightleftharpoons Mn(OH)_4{}^{2-} + 4\,H^+$ | −48.3 |
| $2\,Mn^{2+} + 3\,H_2O \rightleftharpoons Mn_2(OH)_3{}^+ + 3\,H^+$ | −23.9 |
| $2\,Mn^{2+} + 3\,H_2O \rightleftharpoons Mn_2(OH)^{3+} + H^+$ | −10.56 |
| $Mn^{2+} + SO_4{}^{2-} \rightleftharpoons MnSO_4$ | 2.25 |

$ZnSO_4\,|\,MnSO_4$ electrolytes contain $Zn^{2+}$ and $Mn^{2+}$ in a multitude of ion-ligand complexes. To accurately model the transport reactions, knowledge of the complexation is needed. Furthermore, calculation of the pH value, defined as $pH = -\log_{10}(c_{H^+}/c_0)$ requires to solve the detailed speciation Table S1 includes a list of all complex formation reactions and their corresponding thermodynamic stability constants. The transport model for this highly complexed electrolyte is based

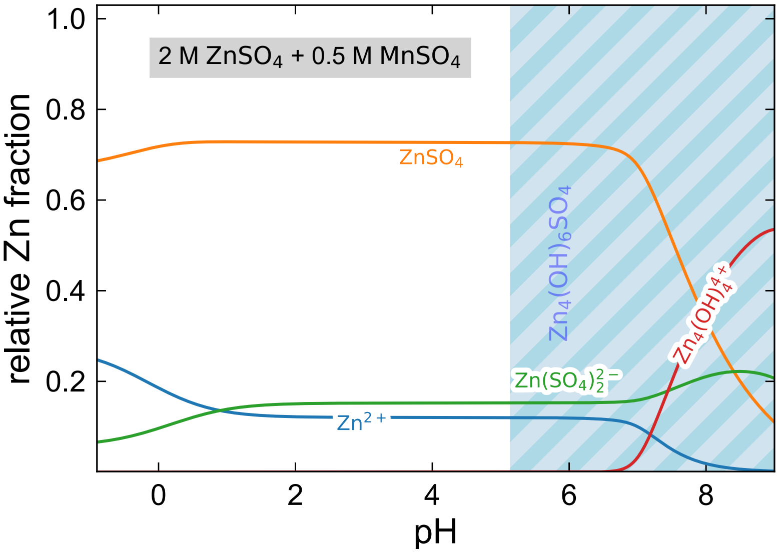


Figure S1: Relative contribution of the individual zinc-ligand complexes as a function of pH. The speciation is calculated for a 2 M $ZnSO_4$, 0.5 M $MnSO_4$ electrolyte. Within this computational titration, the $[{SO_4}^{2-}{}_T]$ concentration is implicitly solved by the charge neutrality of the solution $0 = 2 \cdot \left([{Mn}^{2+}{}_T] + [{Mn}^{2+}{}_T] - [{SO_4}^{2-}{}_T]\right) + [{H}^{+}{}_T]$.

on a set of quasiparticles. The quasi-particle definitions used in this work are as follows

$$[Zn_T^{2+}] = [Zn^{2+}] + \sum_{n=1}^{4}[Zn(SO_4)_n{}^{2\cdot(1-n)}] + \sum_{n=1}^{4}[Zn(OH)_n{}^{2-n}] + 2\cdot\left([Zn_2OH^{3+}] + [Zn_2(OH)_6{}^{2-}]\right) + 4\cdot[Zn_4(OH)_4{}^{4+}] \tag{S1}$$

$$[Mn_T^{2+}] = [Mn^{2+}] + \sum_{n=1}^{4}[Mn(OH)_n{}^{2-n}] + 2\cdot\left([Mn_2OH^{3+}] + [Mn_2(OH)_3{}^{+}]\right) + [MnSO_4] \tag{S2}$$

$$[SO_{4\,T}^{2-}] = [SO_4{}^{2-}] + [HSO_4{}^{-}] + [H_2SO_4] + \sum_{n=1}^{4}[Zn(SO_4)_n{}^{2(1-n)}] + [MnSO_4] \tag{S3}$$

$$[H_T^{+}] = [H^{+}] + [HSO_4{}^{-}] + 2\cdot[H_2SO_4] - [OH^{-}]$$

$$- \sum_{n=1}^{4} n[Zn(OH)n^{2-n}] - [Zn_2OH\,3\,^{+}] - 4 \cdot [Zn_4(OH)_4{}^{4+}] - 6 \cdot [Zn_2(OH)_6]$$

$$- \sum_{n=1}^{4} n[Mn(OH)n^{2-n}] - [Mn_2OH^{3+}] - 3 \cdot [Mn_2(OH)_3{}^{+}] \qquad \text{(S4)}$$

Figure S1 shows the calculated contribution of the individual zinc species for a 2 M $ZnSO_4$, 0.5 M $MnSO_4$ electrolyte.

## 1.2 Cathode Thermodynamics

The cathode thermodynamics are investigated in this work by means of DFT calculations. A condensed discussion of this section can be found in the manuscript (Subsection II A). The cathodic insertion and dissolution potentials are determined by the Gibb's free energy difference $\Delta G$ as $U_i = {}^{-\Delta G}/_{z_i \Delta \mathrm{N}_i}$. We approximate $\Delta G$ from the energy of formation $E_f$ obtained from DFT as

$$\Delta G = E_f + T \cdot \Delta S \tag{S5}$$

, with the entropy $S$ and the systems temperature $T$. We approximate the entropy of the individual states by neglecting the vibrational entropy so that $S \approx S_{\mathrm{conf}}$. The configurational entropy of a specific configuration is here estimated by the Boltzmann formula

$$\begin{aligned} S_{\mathrm{conf}} &= k_{\mathrm{B}} lnW \\ &= k_{\mathrm{B}} \log \binom{N_{\mathrm{lattice}}}{\mathrm{n_{Zn}}, \mathrm{n_H}} \end{aligned} \tag{S6}$$

Here, $k_{\mathrm{B}}$ is the Boltzmann constant and $W$ the number of possible constellations, which is calculated with the binomial coefficient of the number of lattice sites and the number of protons and zinc atoms in the structure. The resulting specific entropy per atom is presented in Figure S2 and is in the range of $0\,\mathrm{k_B T}$ to $1\,\mathrm{k_B T}$.

The difference in Gibbs free energy of the generic insertion following the insertion reaction

$$\underbrace{\mathrm{H_{x_0}Zn_{y_0}Mn_2O_4}}_{\mathrm{A}} + \mathrm{x} \cdot \mathrm{Zn_2}^{+} + \mathrm{y} \cdot \mathrm{H}^{+} + (2 \cdot \mathrm{x} + \mathrm{y}) \cdot \mathrm{e}^{-} \longrightarrow \underbrace{\mathrm{H_{x_0+x}Zn_{y_0+y}Mn_2O_4}}_{\mathrm{B}} \tag{S7}$$

is then calculated as $\Delta G = G_{\mathrm{H_{x_0+x}Zn_{y_0+y}Mn_2O_4}} - G_{\mathrm{H_{x_0}Zn_{y_0}Mn_2O_4}} - \sum_i n_i \Delta\tilde{\mu}_i$, where $\Delta\mu_i$ are the normalized electrochemical potentials of $\mathrm{Zn}^{2+}$ and $\mathrm{H}^{+}$ in the electrolyte. The reservoir used to calculate the chemical potentials is described in a grand-canonical approach in accordance with the computa-

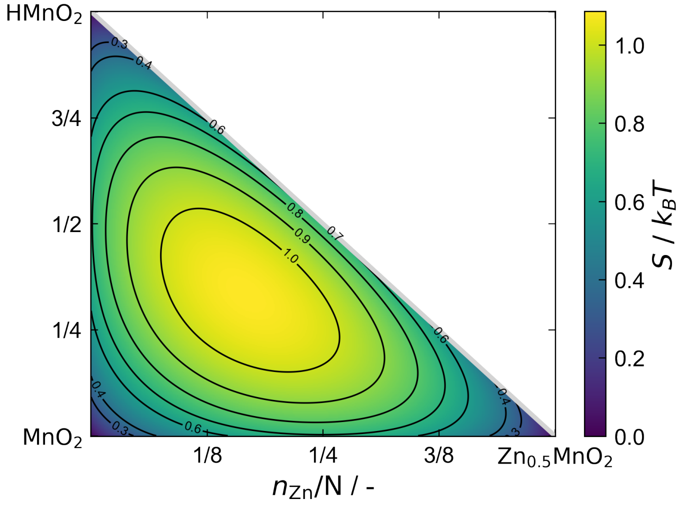


Figure S2: Calculations of the configurational entropy $S^{\text{conf}}$ (Equation S6) as a function of zinc and proton atoms $n_{\text{Zn}}$ and $n_{\text{H}}$ per unit cell N.

tional hydrogen electrode (CHE).[S5] In this work, we use an extension of this concept, as used in Reference S6. The equations for the chemical potential of $H^+$, and the extension of the CHE to the chemical potential of $Zn^{2+}$ are

$$\begin{aligned} \Delta\tilde{\mu}_{\text{H}^+} &= \tilde{\mu}_{\text{H}^+\text{(aq)}} + \tilde{\mu}_{e^-} - \frac{1}{2}E_{\text{H}_2} \\ &= -eU_{\text{SHE}} - k_{\text{B}}T\ln(10)\text{pH}\,, \end{aligned} \tag{S8}$$

$$\begin{aligned} \Delta\tilde{\mu}_{\text{Zn}^{2+}} &= \tilde{\mu}_{\text{Zn}^{2+}\text{(aq)}} + 2\tilde{\mu}_{\text{e}^-} - E_{\text{Zn}} \\ &= -2e\left(U_{\text{SHE}} - U_0\right) - k_{\text{B}}T\ln(a_{\text{Zn}^{2+}})\,. \end{aligned} \tag{S9}$$

(see also Equation (2) and Equation (3)). Subsequently, the difference in Gibbs free energy between state A and B is finally calculated as

$$\begin{aligned} \Delta G = E_{\text{tot}}^{\text{H}_x\text{Zn}_y\text{MnO}_2} - E_{\text{tot}}^{\text{MnO}_2} - T\cdot\left(S_{\text{conf}}^{\text{H}_x\text{Zn}_y\text{MnO}_2} - S_{\text{conf}}^{\text{MnO}_2}\right) \\ - x\cdot\left(E_{\text{tot}}^{\text{Zn(bulk)}} + \Delta\tilde{\mu}_{\text{Zn}^{2+}}\right) - y\cdot\left(\frac{1}{2}E_{\text{tot}}^{\text{H2(gas)}} + \Delta\tilde{\mu}_{\text{H}^+}\right)\,. \end{aligned} \tag{S10}$$

The corresponding charge transferred in this insertion reaction is $z_i = 2\cdot x + y$.

## 1.3 Continuum Model

## 1.4 Cathode Model

We approximate the active mass in the cathodes as spherical particles and use an isotropic diffusion equation to solve the zinc concentration within the particle. The diffusion of zinc within the solid is calculated accordingly:

$$\frac{\partial c_{Zn}}{\partial t} = \frac{1}{r^2}\frac{\partial}{\partial r}\left(D_{solid} \cdot r^2 \frac{\partial c_{Zn}}{\partial r}\right) . \tag{S11}$$

At the particle surface, the zinc concentration increases during insertion and decreases due to the dissolution reaction. At the surface, the boundary condition of the diffusion equation therefore is

$$\left.\frac{\partial c_{Zn}}{\partial t}\right|_{r=r_{cat}} = A_{spec,cat} \cdot (k_{ins} - k_{diss}) . \tag{S12}$$

Here, $k_{ins}$ is the insertion rate (Equation (15)) and $k_{diss}$ is the dissolution rate of $Zn_{0.5}MnO_2$ (Equation (18)) as discussed in the manuscript. The specific surface of the cathode is calculated as a function of the particle radius using our spherical particle assumption.

The volume fraction of the cathode $\epsilon_{cat}$ varies due to the dissolution reaction of $MnO_2$. We solve the volume fraction during the simulation as

$$\frac{\partial \epsilon_{cat}}{\partial t} = V_{Zn_{0.5}MnO_2} \cdot A_{spec,cat} 2 k_{diss} . \tag{S13}$$

Here, $V_{Zn_{0.5}MnO_2}$ is the molar volume of $Zn_{0.5}MnO_2$. The factor of 2 included in this reaction is based on the ratio of Zn and Mn during the dissolution of $Zn_{0.5}MnO_2$ (see Equation (16)). In our model, we use the assumption that there is no volume change during cycling so that $V_{Zn_{0.5}MnO_2} \approx V_{MnO_2}$. During dissolution, we assume, that dissolution occurs at the surface. Therefore, the volume change is happening in the outermost shell. Once the outermost shell is dissolved, we model the dissolution of the second shell and so on. For reasons of numerical stability, we switch to the

dissolution of the next shell once the volume of the previous shell reaches $10\times10^{-5}$ of the original shell volume.

# 2 Cell Parametrization

**Table S2: List of the model parameters. All potentials are relative to the $Zn/Zn^{2+}$ redox couple at standard conditions.**

| Parameter | Description | Value | Unit |
|---|---|---|---|
| $U^0_{Zn}$ | Standard potential of the Zn anode | 0 | V |
| $A_{spec,ano}$ | Specific surface of the Zn anode | $1{\times}10^{6}$ | $m^{-1}$ |
| $k^0_{ano}$ | Rate constant of the anode reaction | $1{\times}10^{-3}$ | $mol\,m^2\,s^{-1}$ |
| $U^0_{ins,Zn^{2+}}$ | $Zn^{2+}$-insertion potential | 1.55 | V |
| $k^0_{ins,Zn^{2+}}$ | Rate constant of the cathodic $Zn^{2+}$ insertion | $1{\times}10^{-5}$ | $mol\,m^2\,s^{-1}$ |
| $U^0_{diss}$ | $ZnMn_2O_4 \cdot H_2O$-dissolution potential | 2.64 | V |
| $k^0_{diss}$ | Rate constant of the cathode dissolution | $0.5{\times}10^{-6}$ | $mol\,m^2\,s^{-1}$ |
| $c_{max,cat}$ | Theoretical concentration limit of the cathode | 28 792 | $mol\,m^{-3}$ |
| $D_{solid}$ | Solid state diffusion coefficient | $1{\times}10^{-15}$ | $m^2\,s^{-1}$ |
| $l_{ano}$ | Anode thickness | 30 | $\mu m$ |
| $\epsilon_{Zn}$ | Zinc volume fraction | 0.2 | - |
| $r^0_{Zn}$ | Initial particle radius in the zinc anode | 75 | $\mu m$ |
| $\epsilon_{ano,\ inactive}$ | Anode inactive volume fraction | 0.4 | - |
| $l_{sep}$ | Separator thickness | 150 | $\mu m$ |
| $\epsilon_{sep}$ | Volume fraction separator | 0.6 | - |
| $l_{cat}$ | Cathode thickness | 66 | $\mu m$ |
| $\epsilon_{MnO_2}$ | Volume fraction of the $MnO_2$ cathode | 0.11 | - |
| $r^0_{MnO_2}$ | Initial particle radius in the $MnO_2$ cathode | 75 | $\mu m$ |
| $\epsilon_{cat,\ \mathit{inactive}}$ | Inactive volume fraction of the cathode (binder,...) | 0.57 | - |
| $c^0_{Zn^{2+}T}$ | Initial electrolyte zinc concentration | 2000 | $mol\,m^{-3}$ |
| $c^0_{Mn^{2+}T}$ | Initial electrolyte manganese concentration | 500 | $mol\,m^{-3}$ |
| $c^0_{SO_4{}^{2-}T}$ | Initial electrolyte sulfate concentration | 2500 | $mol\,m^{-3}$ |
| $K^{ZHS}_{sp}$ | Stability constant of ZHS | 28.4 | - |
| $\delta_0$ | Diffusion length of the ZHS precipitation reaction | 0.3 | $\mu m$ |
| $s_{critical}$ | Oversaturation ratio | 105 | % |

As discussed in the computational section (Section VI), the cell model is parameterized according to recently published designs of $\delta$-$MnO_2$ 2023-type coin cells (see Figure S3). Most of the parameters are chosen to represent the cell design by Chen and coworkers.[S9] However, many of the recently published studies report a design quite similar to their approach. The parameters which were not given in Reference S9 were estimated from other literature, or if not accessible reasonably assumed to match the experimentally observed cycling behavior. In the following, we

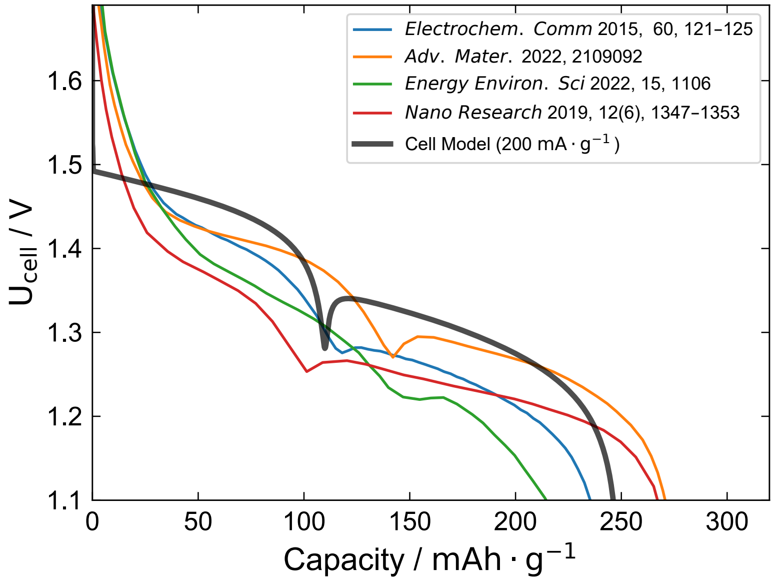


Figure S3: An exemplary comparison of the cell potential for $\delta$-$MnO_2$ 2023-type coin cells during galvanostatic discharge as found in References S7–S10. They were discharged at current densities from 83 mA g$^{-1}$ to 300 mA g$^{-1}$. The cells show different discharge behaviors, however, a voltage dip is observed for all cells between 100 mA h g$^{-1}$ and 150 mA h g$^{-1}$.

will shortly discuss the choice and motivation of the individual parameters of the presented simulation. In Table S2, the individual model parameters are summarized.

We use a 1D+1D volume-averaged cell model. To describe transport within the porous structure of the cell, estimations of the volume fractions of the individual components are needed. The cathode structures used here is a 70:20:10 wt% mixture of $MnO_2$, acetylene black and PVDF. We assume the density of $MnO_2$ as 3704 kg m$^{-3}$ as calculated from the DFT structures. We use a density of acetylene black as $\rho_{\text{ac.black}} = 150\,\text{kg}\,\text{m}^{-3}$ and PVDF of $\rho_{\text{PVDF}} = 1780\,\text{kg}\,\text{m}^{-3}$. The average density of the cathode is then calculated as $\rho_{\text{cathode}} = 1/\sum_i \text{wt}\%_i/\rho_i = 633\,\text{kg}\,\text{m}^{-3}$. This results in volume fractions for the $MnO_2$, acetylene black and PVDF of 13 vol%, 4 vol% and 83 vol%.

Pore volume measurements were conducted by Corpuz et. al. (0.78 cm g$^{-3}$)[S11] and Shen et. al. (0.44 cm g$^{-3}$).[S12] Here, we assume a pore volume of 0.5 cm g$^{-3}$. Using the assumed pore vol-

ume and the average density of the cathode we get a porosity of $\epsilon_{\text{elyt}} = 0.32$. The zinc anode is parameterized as a porous electrode with a volume fraction of the zinc metal of 20 %. Thickness of the separator is assumed as 150 µm in accordance to the literature comparison from Qin et. al.[S13]

The insertion potential of zinc into the $MnO_2$ structure $U^0_{\text{ins,Zn}^{2+}} = 1.55\,\text{V}$, is taken as the average insertion potential for zinc as calculated from the DFT simulations (see Figure 2). The dissolution potential used for the cell simulation is chosen here as 2.64 V, which is similar to the results from DFT (see Table I) but was adjusted slightly to reproduce experimental findings. The rate constants of the insertion and dissolution process are chosen in a way to match the discharge and CV measurements in the literature.

The diffusion coefficient $D_{\text{solid}}$ for zinc within the cathode structure is set to $1\times10^{-11}\,\text{cm}^2\,\text{s}^{-1}$. This is based on GITT measurements which were conducted by Jiang et al. ($2.2\times10^{-15}\,\text{cm}^2\,\text{s}^{-1}$ to $3.1\times10^{-15}\,\text{cm}^2\,\text{s}^{-1}$).[S14] The theoretical capacity of the cathode structure is calculated from the unit cell volume of the $ZnMn_2O_4 \cdot H_2O$, as calculated by DFT (see Figure S5) which gives us $c_{max} = 28.78\,\text{mol}\,\text{L}^{-1}$.

# 3 Simulation Result

In this section, we supply simulation results that support the results shown in the main text in Section III and IV. We show supporting calculations of the electrolyte speciation (Subsection 3.1), supporting material for the DFT calculations (Subsection 3.2), discuss the dynamic results of $H^+$-insertion in our cell model (Subsection 3.3), and show results for full-cell simulations (Subsection 3.4).

## 3.1 Electrolyte Speciation (Thermodynamics)

In the manuscript, we discuss the influence of $H^+$-insertion on the electrolyte equilibrium (see Subsection III B). Here we present the results of an analogous calculation for $Mn^{2+}$-dissolution. We investigate how the electrolyte composition and pH value are influenced by a $Mn^{2+}$-dissolution reaction from the cathode, which reduces the $[H_T^+]$ concentration in the electrolyte. Figure S4 shows the pH value and $Zn^{2+}$ saturation limit in dependence on the amount of $Mn^{2+}$ in the electrolyte which is produced by the dissolution reaction.

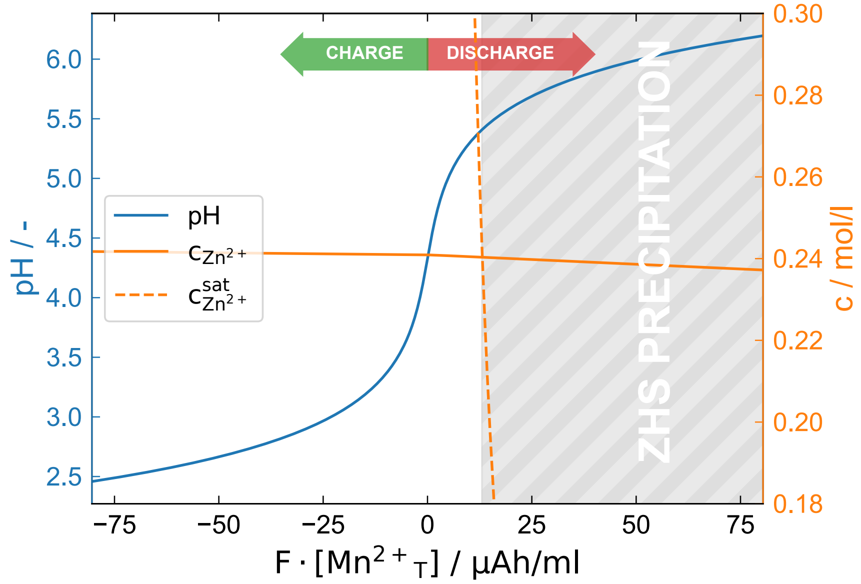


Figure S4: Dependence of electrolyte pH and $Zn^{2+}$ saturation with respect to ZHS precipitation as a function of manganese concentration for a $Mn^{2+}$ reactions in a 2 M $ZnSO_4$, 0.5 M $MnSO_4$ electrolyte. The pH is shown on the left, and zinc concentration and zinc saturation concentration are shown on the right; both are shown as a function of the amount of $Mn^{2+}$ added to the electrolyte. We argue that the dissolution of $Mn^{2+}$ from $MnO_2$ during discharge would result in an decrease of $[H_T^+]$ in the electrolyte.

## 3.2 Electrode Thermodynamics (DFT)

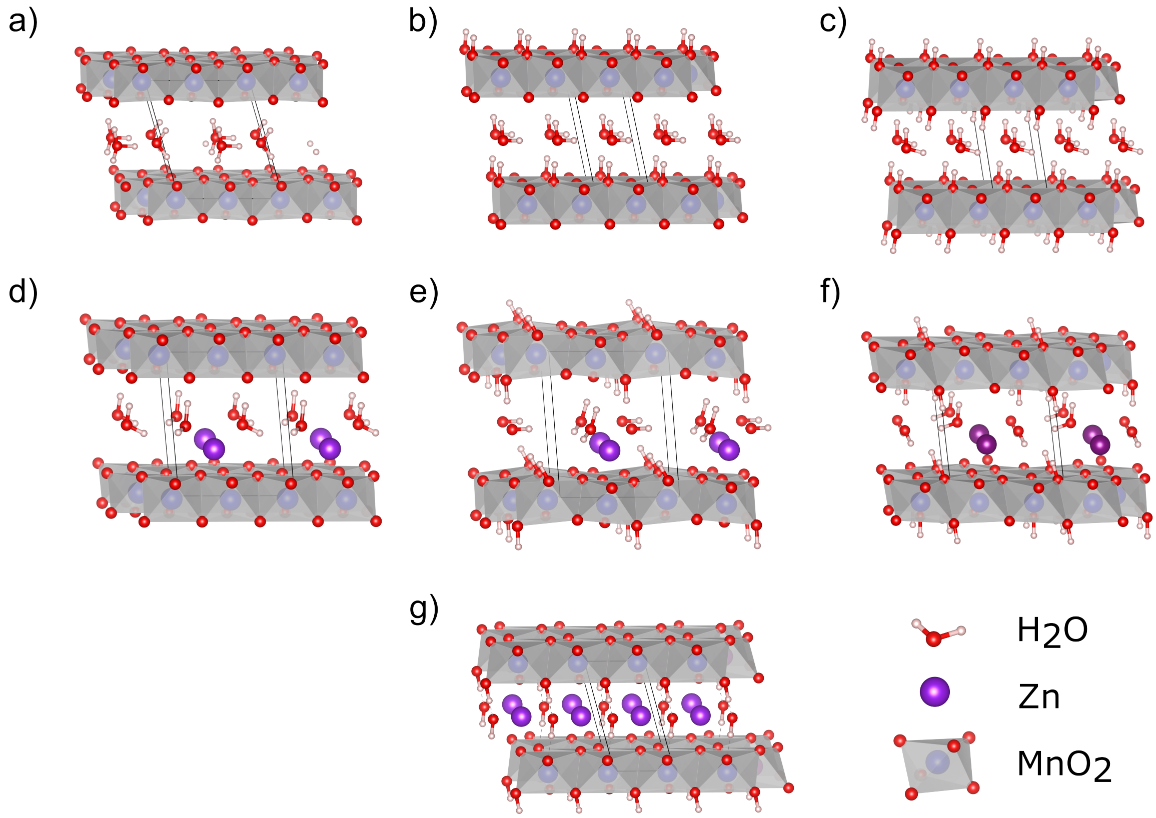


Figure S5: Energetically most stable structures of δ-$MnO_2 \cdot H_2O$ with different $H^+$ and $Zn^{2+}$ contents: (a) $H_{0.25}MnO_2 \cdot H_2O$, (b) $H_{0.5}MnO_2 \cdot H_2O$, (c) $HMnO_2 \cdot H_2O$, (d) $Zn_{0.25}MnO_2 \cdot H_2O$, (e) $H_{0.25}Zn_{0.25}MnO_2 \cdot H_2O$, (f) $H_{0.5}Zn_{0.25}MnO_2 \cdot H_2O$, (g) $Zn_{0.5}MnO_2 \cdot H_2O$.

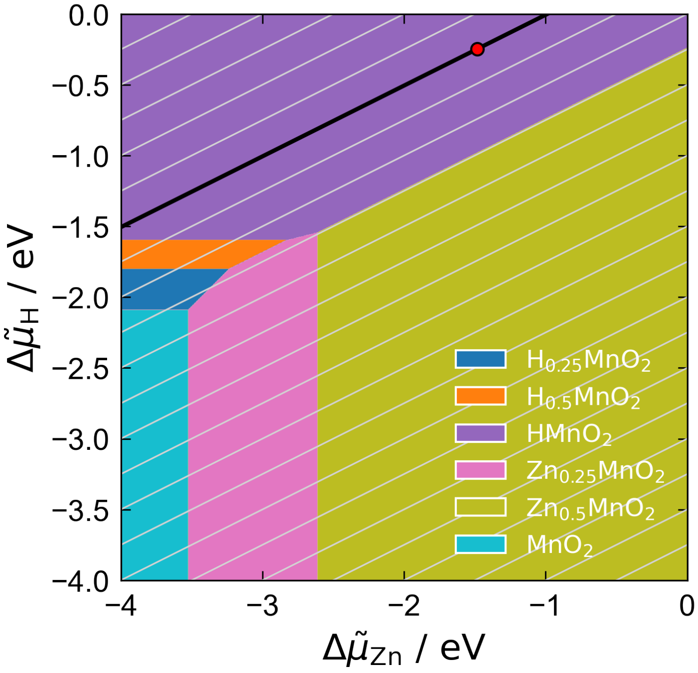


Figure S6: Calculated phase diagrams for hydrogen and zinc intercalation in $\delta$-$MnO_2$ as a function of the respective electrochemical potential. The solid gray lines depict the relative tuning of the electrochemical potentials by an applied electric potential. The red dot and the corresponding black line depict the electrochemical potential in the $ZnSO_4$, $MnSO_4$ electrolyte used here and its electric tuning.

## 3.3 Proton insertion in the first phase (Cell Model)

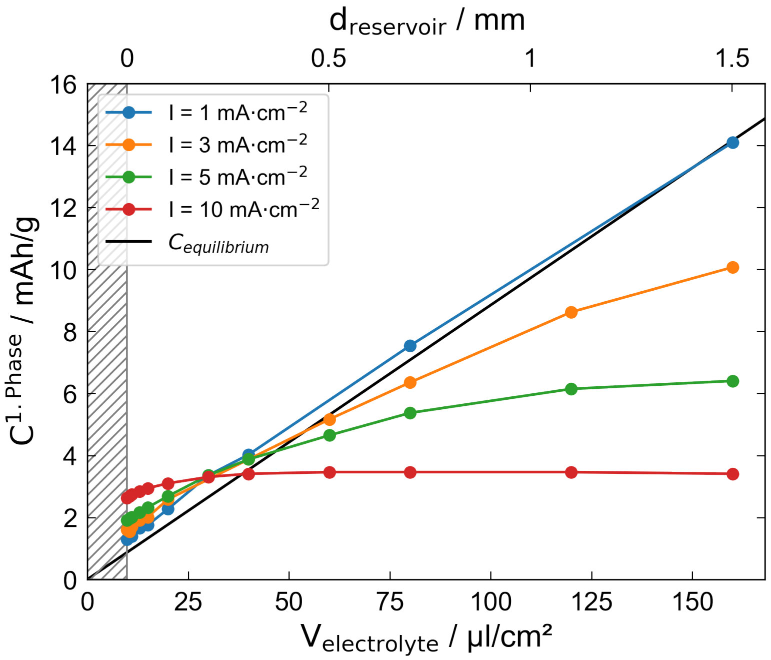


Figure S7: Effective discharge capacity in the first discharge phase. The realized capacity of the first discharge phase (until the onset of ZHS precipitation) is analyzed for $H^+$-insertion. The black line shows the scaling of the equilibrium calculation with electrolyte volume, the dashed region on the left indicates the electrolyte volume contained in the active regions of the cell (anode, separator and cathode).

The calculated electrode potentials indicate that the proton insertion reaction is thermodynamically favorable. However, our equilibrium calculations (Subsection III B) indicate a high sensitivity of the pH of the electrolyte on $H^+$-insertion reaction. In the following, we investigate the influence of $H^+$-insertion in a full-cell model to analyze how concentration gradients and electrolyte volume influences the capacity of the first discharge phase. The saturation limit of ZHS equals a proton-insertion capacity of $52\,\mu A\,h\,mL^{-1}$ as calculated in Subsection III B. Therefore, increasing the amount of electrolyte linearly increases the stability of the electrolyte regarding precipitation. Additional electrolyte volume within the cell might therefore improve electrolyte stability. For the standard cell used in this work, the electrolyte volume in the electrodes and the separator is $93\,\mu L\,cm^{-2}$, which equals an electrolyte loading ratio of $49\,mL\,g^{-1}$ at an active mass loading of $2\,mg\,cm^{-2}$.

However, dynamic behavior, such as supersaturation of the electrolyte, local concentration gradients or the influence of and the interaction with an electrolyte reservoir might further increase the capacity in the first discharge phase. We, therefore, simulate the discharge behavior of a 2023 coin cell for a $H^+$-insertion reaction. To investigate the influence of excessive amounts of electrolyte, we integrate an electrolyte reservoir left of the anode. This allows simulating electrolyte to active mass ratio which is significantly higher than the volume which is necessary to completely wet electrodes and separator. In Figure S7 the precipitation onset is studied for current densities ranging from 1 $mA\,cm^{-2}$ to 10 $mA\,cm^{-2}$ and electrolyte volumes up to 160 $\mu L\,cm^{-2}$. The highest electrolyte volume studied here equals a reservoir thickness of 1.5 mm, which should be higher than the theoretical limit of a 2023-type coin cell. If only a limited amount of electrolyte is used, the capacity is slightly higher than the expectation from equilibrium calculations due to the effect of supersaturation and slow nucleation kinetics. The higher the excess electrolyte, the longer the first discharge phase. However, transport limitations, which are more prominent with high current densities limit the available capacity. At current densities, which are commonly used in experiments, diffusion significantly limits the influence of excessive amounts of electrolyte. Therefore, an insertion reaction of $H^+$ is implausible due to the mismatch of precipitation reactions observed experimentally and the thermodynamically calculated electrolyte stability. The presented simulation results indicate that neither the equilibrium calculation shown in the manuscript (Subsection III B) nor the dynamic behavior during discharge, which was investigated here, can explain the late onset of ZHS for the $H^+$-insertion reaction. Our simulations for the influence of $Mn^{2+}$-dissolution on the precipitation of ZHS, which are in good agreement with the experimental observations (Subsection IV A), can be found in the manuscript in .

## 3.4 Cell-level simulations

This section presents supporting figures of cell-level simulations discussed in the manuscript. Figure S8 shows the pH evolution of the cathode over several cycles. In Figure S9 we show the pH of the electrolyte during the simulated cyclovoltammogram from Figure 8 in the manuscript. Additionally, we investigated an optimized discharge protocol in the manuscript to reduce the cathodic dissolution of $Mn^{2+}$. In Figure S10 and Figure S11 we show the resulting cell potential and current density during the CC-CV discharge for two cases. At a switching voltage of 1.42 V (Figure S10), the discharge potential and current show no signature of ZHS nucleation while at a switching voltage of 1.36 V (Figure S11) the nucleation of ZHS is visible in the current during the potentiostatic phase.

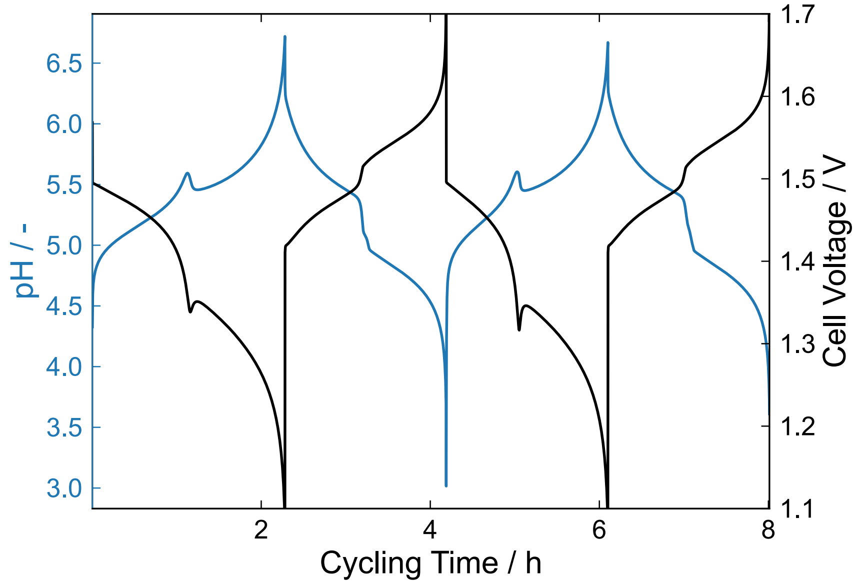


Figure S8: Evolution of the pH at the cathode within the separator during galvanostatic cycling at 8 A $g^{-1}$. The spatially resolved over the complete domain of the cell is presented in 7 of the main document.

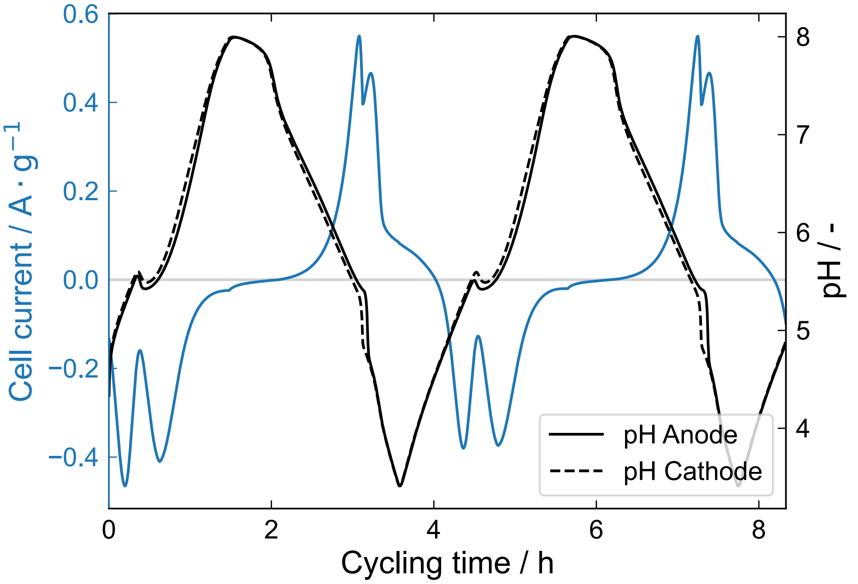


Figure S9: Cell current and electrolyte pH at the anode and cathode during a cyclovoltammogram at a sweep rate of 0.1 mV s$^{-1}$.

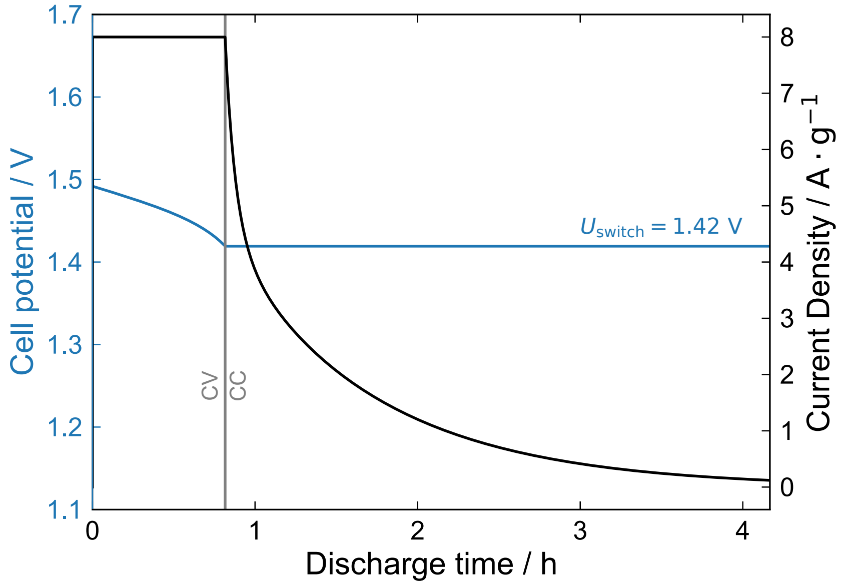


Figure S10: Cell potential and current density for the optimized discharge routine. The galvanostatic discharge is executed until the cell potential reaches 1.42 V. During the potentiostatic discharge, the current linearly decreases.

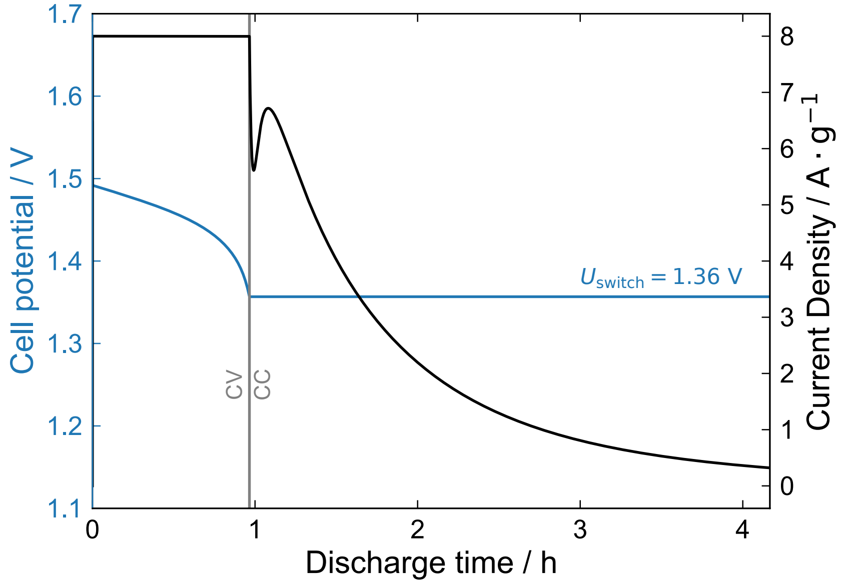


Figure S11: Cell potential and current density for the optimized discharge routine. The galvanostatic discharge is here executed until the cell potential reaches 1.36 V. In this case, the current profile in the potentiostatic region shows the onset of ZHS precipitation which is still occurring here.

# References


(S1) Nordstrom, D. K.; Ball, J. W. WATEQ4F – User's manual with revised thermodynamic data base and test cases for calculating speciation of major, trace and redox elements in natural waters. 1991.

(S2) Ball, J. W.; Nordstrom, D. K. User's Manual for WATEQ4F, with revised thermodynamic data base and test cases for calculating speciation of major, trace, and redox elements in natural waters. *U.S. Geological Survey Water-Resources Investigations Report* **1991**, *91-183*, 1–188.

(S3) R. S. Baes, C.; Mesmer, *The Hydrolysis of Cations*; John Wiley & Sons, 1976.

(S4) Grenthe, I.; Fuger, J.; Konings, R. J. M.; Lemire, R. J.; Muller, A. B.; Nguyen-Trung, C. In *Chemical Thermodynamics: Volume 1*; Wanner, H., Forest, I., Eds.; NUCLEAR ENERGY AGENCY, 2004; Vol. 200; pp 154–155.

(S5) Peterson, A. A.; Abild-Pedersen, F.; Studt, F.; Rossmeisl, J.; Nørskov, J. K. How copper catalyzes the electroreduction of carbon dioxide into hydrocarbon fuels. *Energy and Environmental Science* **2010**, *3*, 1311–1315.

(S6) Liu, X.; Euchner, H.; Zarrabeitia, M.; Gao, X.; Elia, G. A.; Groß, A.; Passerini, S. Operando pH Measurements Decipher H + /Zn 2+ Intercalation Chemistry in High-Performance Aqueous Zn/δ-V 2 O 5 Batteries. *ACS Energy Letters* **2020**, *5*, 2979–2986.

(S7) Alfaruqi, M. H.; Gim, J.; Kim, S.; Song, J.; Pham, D. T.; Jo, J.; Xiu, Z.; Mathew, V.; Kim, J. A layered δ-MnO 2 nanoflake cathode with high zinc-storage capacities for eco-friendly battery applications. *Electrochemistry Communications* **2015**, *60*, 121–125.

(S8) Ren, H.; Zhao, J.; Yang, L.; Liang, Q.; Madhavi, S.; Yan, Q. Inverse opal manganese dioxide constructed by few-layered ultrathin nanosheets as high-performance cathodes for aqueous zinc-ion batteries. *Nano Research* **2019**, *12*, 1347–1353.

(S9) Chen, H.; Dai, C.; Xiao, F.; Yang, Q.; Cai, S.; Xu, M.; Fan, H. J.; Bao, S. Reunderstanding the Reaction Mechanism of Aqueous Zn–Mn Batteries with Sulfate Electrolytes: Role of the Zinc Sulfate Hydroxide. *Advanced Materials* **2022**, 2109092.

(S10) Yang, H.; Zhou, W.; Chen, D.; Liu, J.; Yuan, Z.; Lu, M.; Shen, L.; Shulga, V.; Han, W.; Chao, D. The origin of capacity fluctuation and rescue of dead Mn-based Zn–ion batteries: a Mn-based competitive capacity evolution protocol. *Energy & Environmental Science* **2022**, *15*, 1106–1118.

(S11) Corpuz, R. D.; Juan, L. M. Z. D.; Praserthdam, S.; Pornprasertsuk, R.; Yonezawa, T.; Nguyen, M. T.; Kheawhom, S. Annealing induced a well-ordered single crystal δ-MnO2 and its electrochemical performance in zinc-ion battery. *Scientific Reports* **2019**, *9*, 15107.

(S12) Shen, H.; Liu, B.; Nie, Z.; Li, Z.; Jin, S.; Huang, Y.; Zhou, H. A comparison study of MnO 2 and Mn 2 O 3 as zinc-ion battery cathodes: an experimental and computational investigation. *RSC Advances* **2021**, *11*, 14408–14414.

(S13) Qin, Y.; Liu, P.; Zhang, Q.; Wang, Q.; Sun, D.; Tang, Y.; Ren, Y.; Wang, H. Advanced Filter Membrane Separator for Aqueous Zinc-Ion Batteries. *Small* **2020**, *16*, 2003106.

(S14) Jiang, Y.; Ba, D.; Li, Y.; Liu, J. Noninterference Revealing of "Layered to Layered" Zinc Storage Mechanism of δ-MnO 2 toward Neutral Zn–Mn Batteries with Superior Performance. *Advanced Science* **2020**, *7*, 1902795.
